# Supplementary material for: Mitigating Sybil Attacks on Differential Privacy based Federated Learning
Source: arXiv:2010.10572 source file (2020-10-20)
Supplement: Supplementary file 1 [file appendix.tex]

\appendices
\section{Proof of the First Zonklar Equation}
Appendix one text goes here.

% you can choose not to have a title for an appendix
% if you want by leaving the argument blank
\section{}
Appendix two text goes here.
